# Supplementary material for: Exploring Perception-Based Techniques for Redirected Walking in VR: A Comprehensive Survey
Source: arXiv:2505.16011 source file (2025-05-21)
Supplement: Supplementary file 1 [file suppMaterial.pdf]

# Supplementary Material

## 1 Exploring Use Cases of the Taxonomy

We intend for our taxonomy to serve as both a classification system for existing works and a framework for modular construction of new RDW algorithms. We illustrate how to use the taxonomy to develop new RDW techniques, or to guide the selection and implementation of an existing RDW algorithm.

### 1.1 Creating a New RDW Algorithm

First the researcher should consider what use-case their algorithm is intended for, what VEs and PEs it is intended to operate within, and any improvements they seek to explore with their new technique. Then with those considerations they should follow through the framework to help determine what components to construct their algorithm with.

Any perception-based RDW algorithm needs to have Gains, Target Heading Calculation, and a method for applying gains, alongside optional enhancements under certain circumstances. First, the reader should consider what gains (detectability and type) are applicable for their use cases: for instance, if one wants to implement a technique to subtly guide users, they would want to choose subtle gains, as defined by detectability thresholds (see Sect. 5, Table 1). The reader can select one or more types of gains (rotation, curvature, translation, and/or bending). In most cases, using multiple types of gains seems to be more useful than focusing on one type [1, 2, 7, 8], this seems logical since different gain types correspond to different motion types therefore supporting more gain types enables redirection in more scenarios. For example rotation gains apply when the user is not walking but is rotating in place, where curvature gains apply when users are walking. Many existing algorithms opt for using at least curvature and rotation gains, though some also add translation gains to this. Other types of gains, such as jumping, can be incorporated, though are often more tailored to specific use cases. If the reader wants an algorithm that expands motions beyond walking on a flat 2D plane then some of these gains can be useful, such as jumping gains to enable jumping motions or slope gains for environments that involve motion along slopes.

Afterward, the reader should select the target heading calculation type best suiting their application (see Sec. 6): avoidance-based algorithms tend to work better than steering, especially in complex physical environments (see Sec. 6.2). However, if the application contains many interaction targets supporting passive haptics, an alignment algorithm would make more sense (see Sec. 6.3). Otherwise, if the algorithm will be used in simple PEs, without many obstacles, and the user wants a simple technique; steering techniques may be more beneficial for the ease of implementation (see Sec. 6.1).

Next, considering gain application type (reactive, predictive, scripted) (see Sec. 7): if the algorithm is applied to a simple maze environment or a guided tour with fixed paths within a specific, fixed, known physical environment, a scripted technique that can calculate the ideal gains to use at any point is recommended (see Sec. 7.3). Implementing the algorithm, using a predictive approach, would leverage predicted locomotion for better redirection than reactive techniques at the

cost of more complicated development and computation (see Sec. 7.2). Predictive techniques that are not RL-based also require VE constraints. However, the simplest and most broadly applicable choice is a reactive approach, simply reacting to the user's current state without considering future locomotion (see Sec. 7.1).

Once these choices are made, the reader can consider any optional enhancements to the technique that may prove beneficial (see Sec. 8). For example, if the application is intended to support multiple users in the same physical space, then implementing one of the techniques for enabling multi-user awareness and collision avoidance is recommended. Also, if further hiding the RDW technique during application is intended, then considering gain masking techniques, such as distractors during redirection events, would be relevant. Although these techniques may be less useful for scripted techniques if the redirection can be accomplished with gains within acceptable thresholds without inducing extra head movements. However, if the technique can be custom built for the VR experience and the reader can budget the effort to do so a technique involving distractors or non-visual stimuli can improve the effectiveness of non-scripted techniques while also allowing the technique to be integrated as a seamless immersive component of the experience. Further the reader can consider if the environment the technique will be used within could be irregularly shaped as incorporating enhancements for irregular environments can improve the effectiveness and applicability of the technique to more spaces.

Here we outline some sample choices following this procedure. If the researcher intends for their RDW algorithm to operate only or mostly in complex PEs potentially of non-standard shape or containing interior obstacles, then they would want to consider how to handle this during the construction of the algorithm: an obvious choice is to consider existing enhancements outlined in general enhancements for irregular environments (see Sec. 8.4). While considering these enhancements, they would also want to account for target orientation calculation type for their technique as it would influence the ease of implementing complex environment support: avoidance and alignment techniques show improved support for irregular environments over steering techniques, with mostly only machine learning-based steering techniques offering support for irregular environments. The researchers could consider an alignment technique with enhancements to improve irregular environment support. From here they could decide on gains and gain application type.

Another application for the taxonomy is creating a technique for a guided tour with haptic interaction targets. While there are many scripted techniques effective for guided tours, the researchers could create a new scripted technique (as is typical for guided interactions where locomotion can be limited and pre-planned), and use alignment target heading calculation. While our taxonomy identifies such a technique would be effective for this scenario, few exist within the corpus, highlighting an area for further work. The framework helps guide to the selection of this combination by showing that scripted techniques are best for these pre-planned locomotion applications, and that alignment is the best target heading calculation for passive haptic support.

Potential new techniques that can be developed under this taxonomy include: a predictive alignment technique leveraging locomotion predictions to improve the alignment metric, multi-user alignment techniques that incorporate collision avoidance between multiple users either by finding a balance between collision avoidance and alignment metric or defining a new alignment metric that incorporates other users, and a new scripted avoidance technique leveraging APFs by discretizing the physical environment to calculate the avoidance forces at specific points and using these values to create a mapping between the physical and virtual environments.

## 1.2 Selecting an Existing RDW Algorithm

As with designing a new algorithm the reader should consider the same questions about their intended use case for the RDW algorithm. Following the same process as above for selecting gains, target orientation calculation, gain application, and general enhancements to be applied. Then using this they can look through the works in the corpus and how they are categorized to find a fitting algorithm (see Sec. 6 and Sec. 7).

Here we highlight some examples of this process. The reader wants an algorithm to support multiple-users within their application. Then a good starting point is to consider what techniques are mentioned in the general enhancement section on multi-user support. Furthermore, APF avoidance techniques show good performance for multi-user support as such considering avoidance techniques could also be a good starting point. Looking at Table 2 in Sec. 6, users could consider APF-RDW as outlined in [1, 5], or Push/Pull Reactive (P2R) as defined in [8].

Similarly, a user wanting a technique for use navigating their maze-like VE would want to consider predictive techniques since graph based predictive techniques can leverage the maze-like constrained VE. Looking at Table 3 in Sec. 7, users could consider techniques from [3, 4, 6, 9, 10]. They could then use other factors of import to the VR application to narrow down which technique to select, as some methods here are avoidance and some are steering-based, with differing pros and cons.

When designing a VR experience using perception-based RDW for locomotion, developers should first clearly define their requirements for RDW. Next, check if an existing technique meets these needs using the provided framework. If no suitable technique exists, developers must assess whether they have the resources to create of modify a technique to fit their specifications, keeping in mind trade-offs between effectiveness, ease of implementation, and available resources. Overall, this taxonomy offers a modular framework that assists in deciding whether to develop a new RDW technique or incorporate an existing technique into the application.

# References


[1] Eric R. Bachmann, Eric Hodgson, Cole Hoffbauer, and Justin Messinger. Multi-user redirected walking and resetting using artificial potential fields. *IEEE Transactions on Visualization and Computer Graphics*, 25(5):2022–2031, 2019.

[2] Ze-Yin Chen, Yi-Jun Li, Miao Wang, Frank Steinicke, and Qinping Zhao. A reinforcement learning approach to redirected walking with passive haptic feedback. In *2021 IEEE International Symposium on Mixed and Augmented Reality (ISMAR)*, pages 184–192, Bari, Italy, 2021. IEEE.

[3] Ben J. Congdon and Anthony Steed. Monte-carlo redirected walking: Gain selection through simulated walks. *IEEE Transactions on Visualization and Computer Graphics*, 29(5):2637–2646, 2023.

[4] Cheng-Wei Fan, Sen-Zhe Xu, Peng Yu, Fang-Lue Zhang, and Song-Hai Zhang. Redirected walking based on historical user walking data. In *2023 IEEE Conference Virtual Reality and 3D User Interfaces (VR)*, pages 53–62, Shanghai, China, 2023. IEEE.

[5] Justin Messinger, Eric Hodgson, and Eric R. Bachmann. Effects of tracking area shape and size on artificial potential field redirected walking. In *2019 IEEE Conference on Virtual Reality and 3D User Interfaces (VR)*, pages 72–80, Osaka, Japan, 2019. IEEE.

[6] Thomas Nescher, Ying-Yin Huang, and Andreas Kunz. Planning redirection techniques for optimal free walking experience using model predictive control. In *2014 IEEE Symposium on 3D User Interfaces (3DUI)*, pages 111–118, Minneapolis, MN, USA, 2014. IEEE.

[7] Sharif Razzaque. *Redirected walking*. PhD thesis, University of North Carolina at Chapel Hill, USA, 2005. AAI3190299.

[8] Jerald Thomas and Evan Suma Rosenberg. A general reactive algorithm for redirected walking using artificial potential functions. In *2019 IEEE Conference on Virtual Reality and 3D User Interfaces (VR)*, pages 56–62, Osaka, Japan, 2019. IEEE.

[9] Markus Zank and Andreas Kunz. Optimized graph extraction and locomotion prediction for redirected walking. In *2017 IEEE Symposium on 3D User Interfaces (3DUI)*, pages 120–129, Los Angeles, CA, USA, 2017. IEEE.

[10] Michael A. Zmuda, Joshua L. Wonser, Eric R. Bachmann, and Eric Hodgson. Optimizing constrained-environment redirected walking instructions using search techniques. *IEEE Transactions on Visualization and Computer Graphics*, 19(11):1872–1884, 2013.
